# Supplementary material for: First-principles study of the electronic structure, Z2 invariant and quantum oscillation in the kagome material CsV3Sb5
Source: arXiv:2410.13162 source file (2024-10-17)
Supplement: Supplementary file 1 [file final_CSV_supplementry.pdf]

# Supplemental Materials on "First-principles study of the electronic structure, $Z_2$ invariant and Quantum oscillation in the kagome material $CsV_3Sb_5$"

Shalika R. Bhandari,[1,2,*] Mohd Zeeshan,[3] Vivek Gusain,[3] Keshav Shrestha,[4] and D. P. Rai[5,†]

[1] *Department of Physics, Bhairahawa Multiple Campus, Tribhuvan University, siddarthanagar-32900, Bhairahawa, Nepal*
[2] *Leibniz Institute for Solid State and Materials Research, IFW Dresden, Dresden-01609, Germany*
[3] *Department of Physics,Indian Institute of Technology, Hauz Khas, New Delhi-110016, India*
[4] *Department of Chemistry and Physics, West Texas A and M University, Canyon, Texas 79016, USA*
[5] *Department of Physics, Mizoram University, Aizawl 796004, India*

(Dated: October 15, 2024)

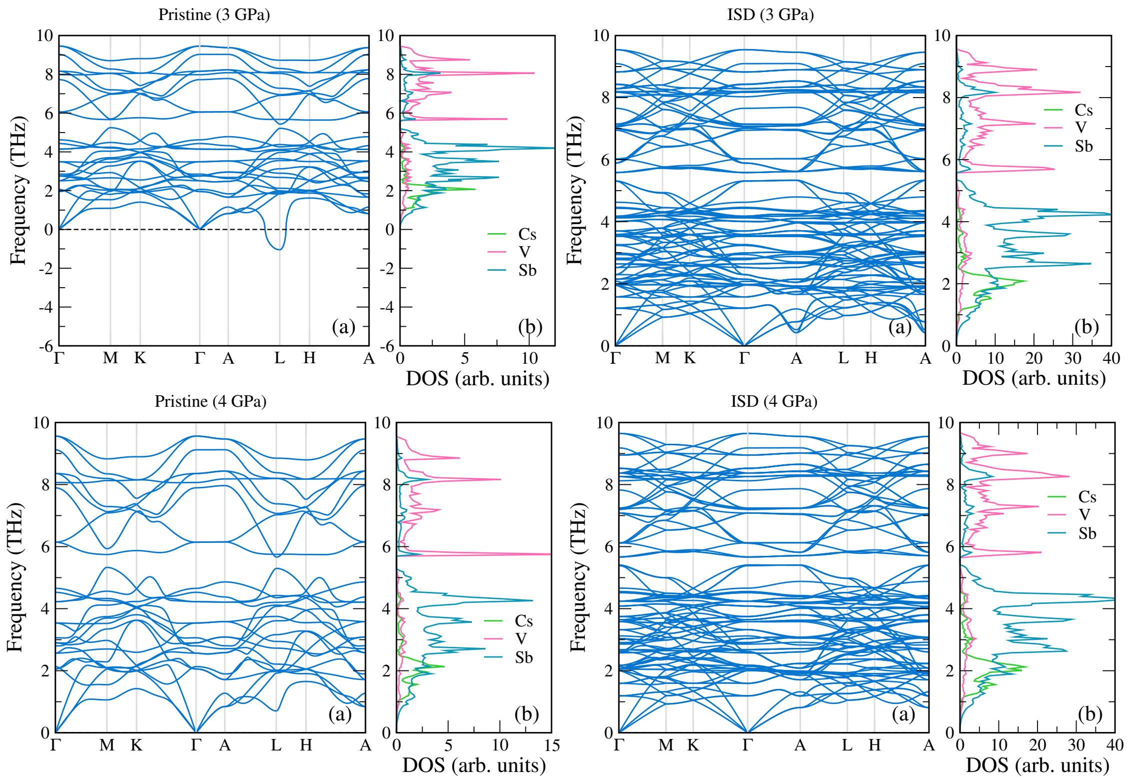


FIG. 1. Phonon dispersions bands structure and density of states of pristine and 2×2×2 ISD state of $CsV_3Sb_5$ at different pressure.

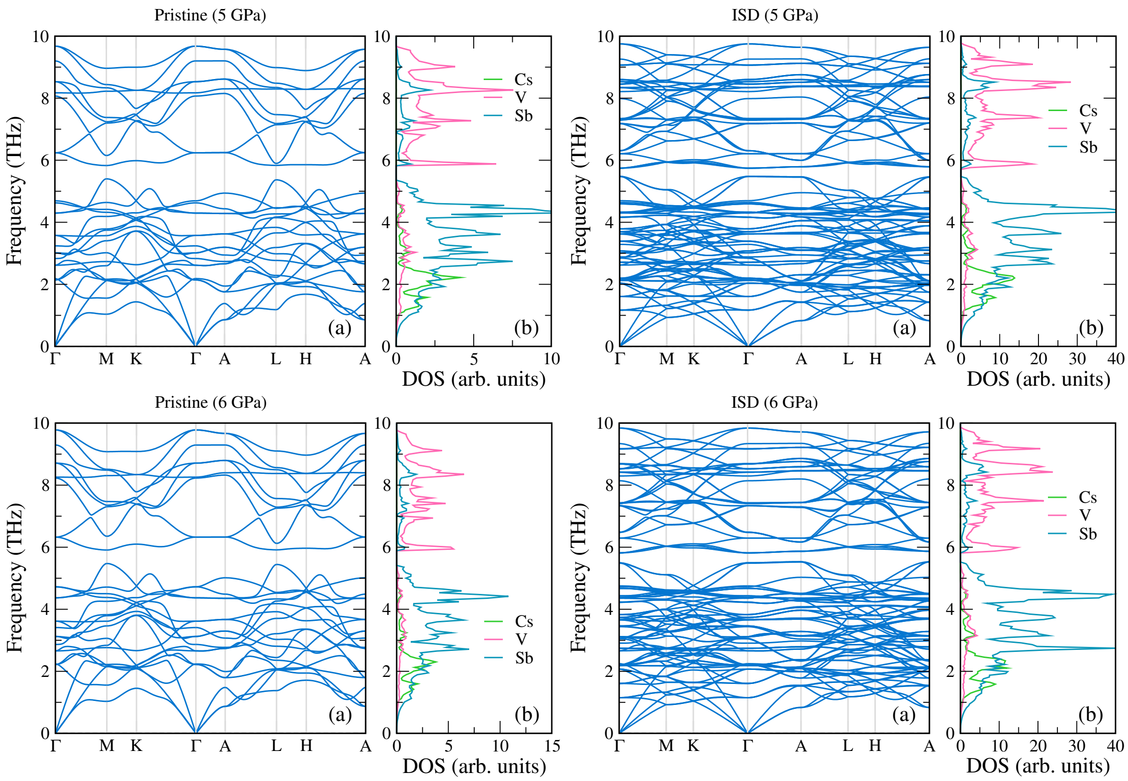


FIG. 2. Phonon dispersions bands structure and density of states of pristine and 2×2×2 ISD state of $CsV_3Sb_5$ at different pressure.

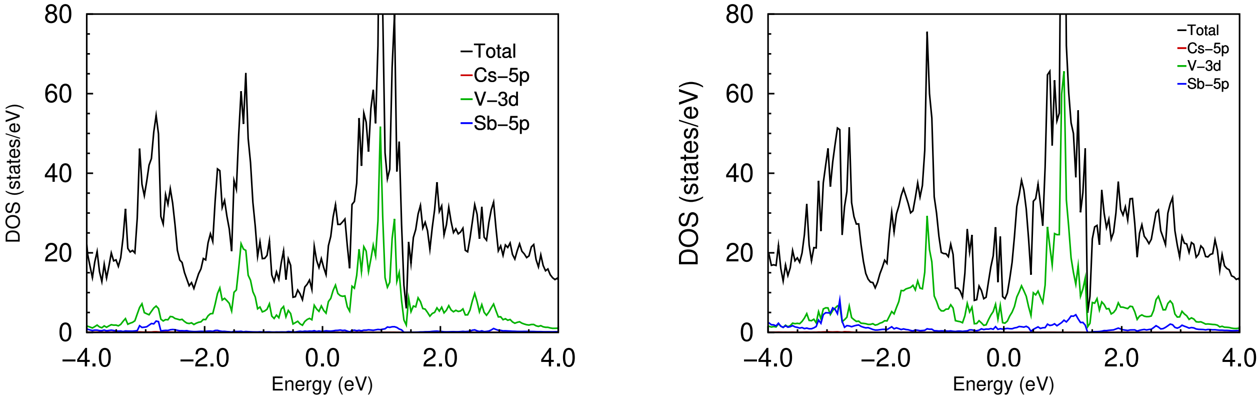


FIG. 3. DFT calculated density of states (DOS) for Pristine and 2×2×1 CDW phase of $CsV_3Sb_5$.

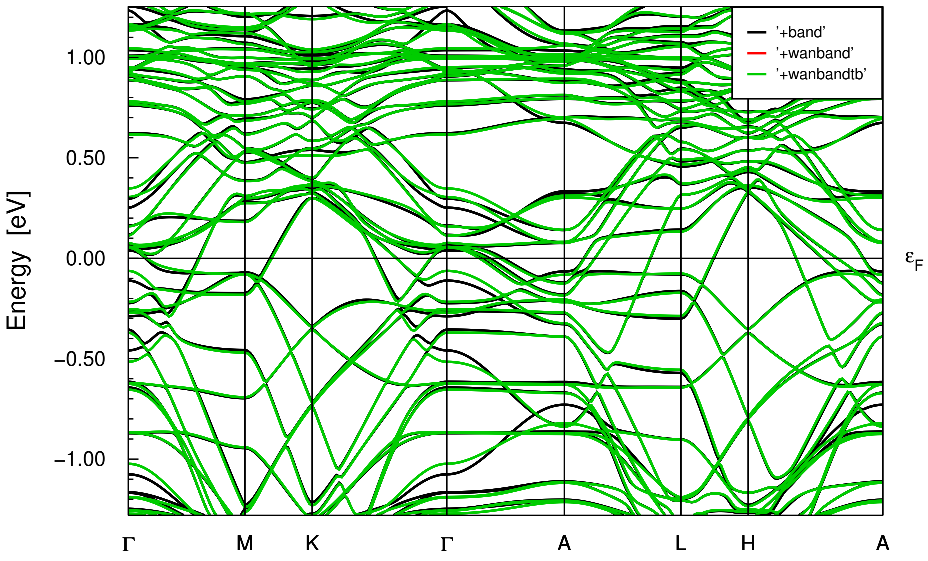


FIG. 4. Wannier model bands (red/green) fitted from fplo for 2×2×2 ISD state of $CsV_3Sb_5$.

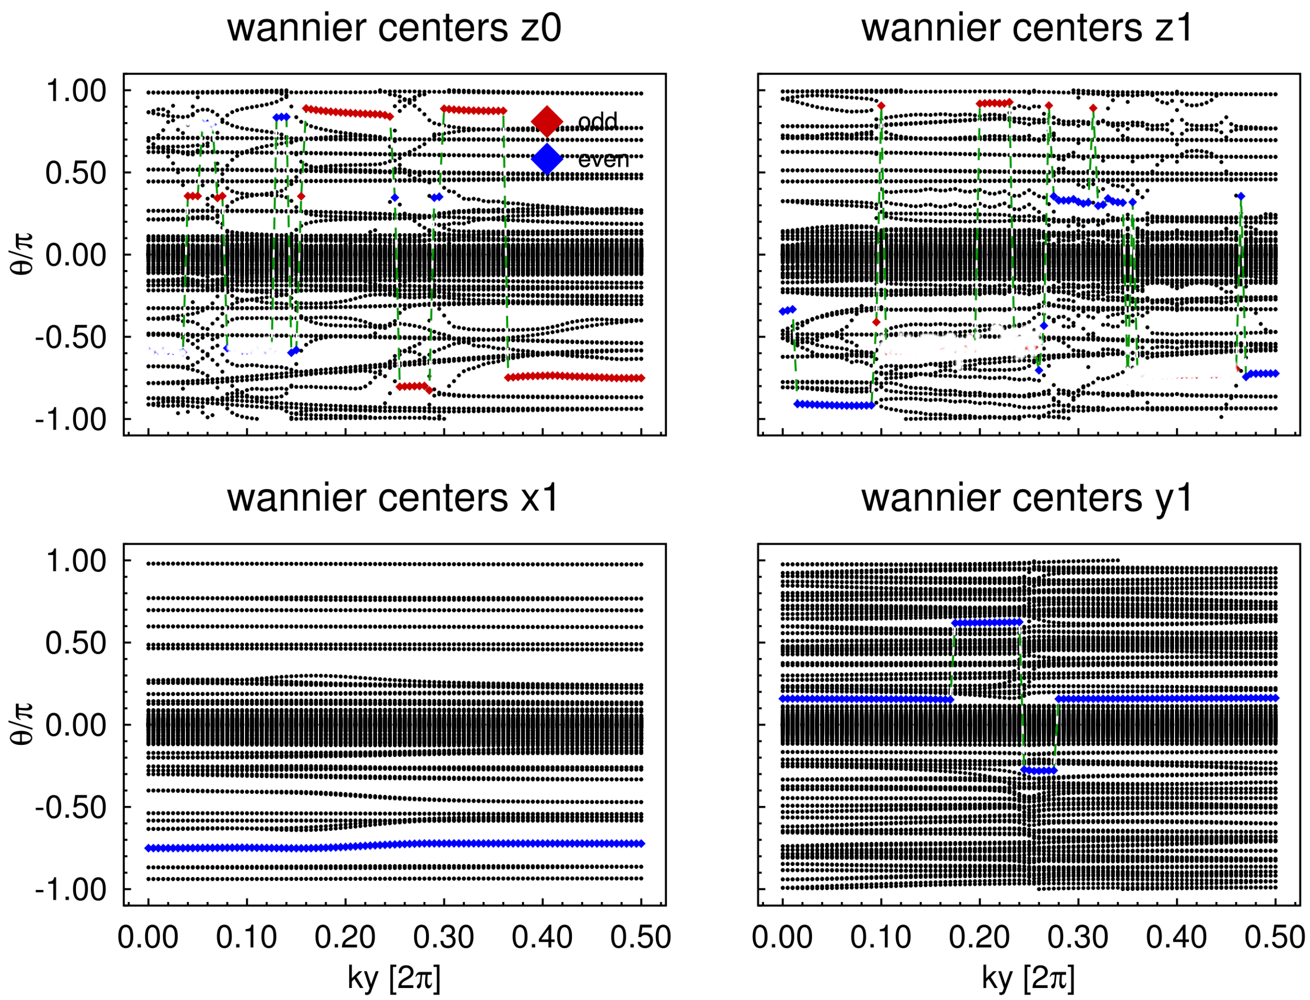


FIG. 5. Non trivial $Z_2$ invariant Wannier center curve representation in the plane spanned by the TRIM for 2×2×2 ISD structure of $CsV_3Sb_5$. Wannier centers and reference line for homo 268. The $x_1$,$y_1$ and $z_1$ planes have zero $Z_2$ invariant, while plane $z_0$ is non-trivial.

TABLE I. Calculated lattice parameters for pristine and ISD $CsV_3Sb_5$ in $P6/mmm$ (191) symmetry. The values in parentheses are from the experiment.

| | Pristine | | ISD | |
|---|---|---|---|---|
| Pressure | a (Å) | c (Å) | a (Å) | c (Å) |
| 0 GPa | 5.43 (5.44) | 9.21 (9.33) | 10.89 (10.87) | 9.30 (9.33) |
| 2 GPa | 5.41 | 8.61 | 10.82 | 8.63 |
| 3 GPa | 5.40 | 8.46 | 10.80 | 8.47 |
| 4 GPa | 5.38 | 8.34 | 10.77 | 8.35 |
| 5 GPa | 5.37 | 8.24 | 10.75 | 8.25 |
| 6 GPa | 5.36 | 8.16 | 10.72 | 8.17 |
